# Supplementary material for: Tight Dimension Independent Lower Bound on the Expected Convergence Rate for Diminishing Step Sizes in SGD
Source: arXiv:1810.04723 source file (2019-11-08)
Supplement: Supplementary file 1 [file appendix.tex]

\section*{Appendix}
